# Supplementary material for: Fault-Tolerant Control of Degrading Systems with On-Policy Reinforcement Learning
Source: arXiv:2008.04407 source file (2020-08-10)
Supplement: Supplementary file 1 [file appendix.tex]

\section{System Operation}

Algorithm \ref{alg:system} describes the logic governing system dynamics.

\begin{algorithm}[ht]
\caption{Fuel tank system model operation}
\label{alg:system}
\begin{algorithmic}[1]
\Require engine fuel demands $\vec{d}$
\Require tank pump capacities $\vec{p}$
\Require valve resistances $\vec{r_v}$
\Require tank heights $\vec{h}$
\Require tank cross sections $\vec{c}$
\Require gravitational potential $g$
\Procedure{system}{state $\vec{x} \in \mathcal{R}^6$, action $\vec{u} \in \{0, 1\}^6$}
    \State Initialize rate of change of state $\delta \vec{x} \gets \vec{0}$
    \State \Comment{Calculate pump flow rates}
    \State $d_l \gets$ total left engine demands
    \State $d_r \gets$ total right engine demands
    \State $l, r \gets$ median left, right tanks
    \While{$d_l > 0, d_r > 0$}
        \State $supply_l \gets \min(\vec{x}[l], \vec{p}[l], d_l)$
        \State $supply_r \gets \min(\vec{x}[r], \vec{p}[r], d_r)$
        \State $d_l \gets d_l - supply_l$
        \State $d_r \gets d_r - supply_r$
        \State $\delta \vec{x}[l] \gets \vec{x}[l] - supply_l / \vec{c}[l]$
        \State $\delta \vec{x}[r] \gets \vec{x}[r] - supply_r / \vec{c}[r]$
        \State $l, r \gets l-1, r+1$
    \EndWhile
    \State \Comment{Calculate valve flow rates $\vec{f}$}
    \State conduit potential $V_{ref} \gets g\cdot\max(\vec{x}\; where\; \vec{u} > 0)$
    \State source tanks where $g \cdot \vec{x} = V_{ref}$
    \State sink tanks where $g \cdot \vec{x} < V_{ref}$
    \State sink tank potential $\vec{V_s}: g\cdot x < V_{ref}$
    \State $\vec{f_{sink}} = + (V_{ref} - \vec{V_s}) / \vec{r_v}$
    \State total flux: $f = \sum{\vec{f_{sink}}} = \sum{\vec{f_{source}}}$
    \State $\vec{f_{source}} = -f \cdot r_v[\mathrm{tank}]^{-1}/\sum{\vec{r_v}[\mathrm{sources}]^{-1}}$
    \State $\delta \vec{x} \gets \delta \vec{x} + [\vec{f_{sink}}, \vec{f_{source}}] / \vec{c}$
    \State \textbf{return} $\delta \vec{x}$
\EndProcedure
\end{algorithmic}
\end{algorithm}

\section{Parameters}

\subsection{System constants}

The following system parameters were used in this paper.

\begin{description}
    \item [Gravitational potential /$ms^{-2}$] $g = 10.$
    \item [Tank heights $/m$] $\vec{h} = 1$ for all tanks.
    \item [Tank cross sections /$m^2$] $\vec{c} = 1$ for all tanks.
    \item [Valve resistances /$\Omega$] $\vec{r_v} = 100$ for all valves,
    \item [Pump capacities /$m^3 s^{-1}$] $\vec{p} = 0.1$ for all pumps.
    \item [Engine demands /$m^3 s^{-1}$] $\vec{e} = 0.025$ for all engines
\end{description}

\subsection{Hyperparameters}

Hyperparameter grid search for the fuel tanks model was conducted over the following grid:

\begin{description}
    \item [Architecture] \texttt{(32, 32), (32, 32, 32), (64,64),\\
    (128, 128), (256, 256), (512, 512)}
    \item [Learning rate] $10^{-2}$, $5 \times 10^{-3}$, $10^{-3}$
    \item [Activation] \texttt{ReLU}, $\tanh{}$
\end{description}

Models had 12 inputs and 6 outputs corresponding to the mapping $x_t \times u_t \rightarrow x_{t+1}$. Evaluation was based on average metrics of 3 fold cross validation on 2950 samples. The mean coefficient of determination over the 6 outputs was used as the evaluation metric. All other model parameters (optimizer, batch size) were kept at defaults as specified in the \texttt{Scikit-Learn MLPRegressor} class (\cite{scikit-learn}).

The reinforcement learning agent using the PPO algorithm was implemented using the \texttt{Stable-Baselines} library (\cite{stable-baselines}). It had the following parameters:

\begin{description}
    \item [Learning rate] $10^{-2}$
    \item [Update interval] $t_{update} = 128$
    \item [Architecture] A shared policy $\pi(x)$ and value $V(x)$ network. First two layers of 64 units are shared. Then two branches each of two layers of 16 units each. $\tanh{}$ activation is used throughout.
\end{description}

% \subsection{Source Code}

% Source code for this work can be found at \url{https://git.isis.vanderbilt.edu/ahmedi/airplanefaulttolerance/-/tree/ifac2020}
